# Supplementary material for: Replay the Curvature: Accurate and Scalable NVFP4 Quantization for Large Language Model Inference
Source: arXiv:2609.36654 source file (2026-09-29)
Supplement: Supplementary file 1 [file qwen_examples.tex]

% Qwen qualitative examples are integrated by dataset in supplementary_details.tex.
